# Supplementary material for: Keyframe-based monocular SLAM: design, survey, and future directions
Source: arXiv:1607.00470 source file (2018-01-07)
Supplement: Supplementary file 1 [file Appendix.tex]

\section{Appendix}
\newgeometry{left=1.5cm,bottom=2cm,top=1.5cm}
	\definecolor{gray}{rgb}{0.75, 0.75, 0.75}
	\begin{singlespace}
        \begin{table}[!h]
			\caption{List of different monocular SLAM system. Keyframe-based approaches are highlighted
            in a gray color.} \label{tab:allcontributions}
			\begin{center}
			\begin{tabular}{c p{9cm} c c l }
				\hline
				\textbf{Year} &\textbf{Name} & \textbf{Method} & \textbf{Type}& \textbf{Reference}  \\
				\hline
				2003&Real-time simultaneous localization and mapping with a single camera
                &filter      &indirect &\cite{davison_2003_ICCV}\\
				\hline
				2004&Simultaneous localization and mapping using multiple view feature descriptors
                &filter      &indirect &\cite{meltzer_2004_IROS}\\
				\hline
				2004&Real-Time 3D SLAM with Wide-Angle Vision
                &filter      &indirect &\cite{davison_2004_IFAC}\\
				\hline
				2005&Real-Time Camera Tracking Using a Particle Filter
                &filter      &indirect &\cite{pupilli_2005_BMVC}\\
				\hline
				2005& CV-SLAM&filter&indirect&\cite{jeong_2005_IROS}\\
				\hline
				\rowcolor{gray}
				2006& Real-time Localization and 3D Reconstruction&keyframe
                &indirect&\cite{mouragnon_2006_CVPR} \\
				\hline
				2006&Scalable Monocular SLAM                                                                &filter      &indirect &\cite{eade_2006_CVPR}\\
				\hline
				2006&Real-Time Monocular SLAM with Straight
                Lines&filter&indirect&\cite{smith_2006_BMVC}\\
				\hline
				2006&Real-Time and Robust Monocular SLAM Using Predictive Multi-resolution
                Descriptors&filter&indirect&\cite{chekhlov_2006_CAVC}\\
				\hline
				2007&Monocular-vision based SLAM using Line
                Segments&filter&indirect&\cite{lemaire_2007_ICRA}\\
				\hline
				2007&MonoSLAM
                &filter      &indirect &\cite{davison_2007_PAMI}\\ 
				\hline
				\rowcolor{gray}
				2007& Parallel Tracking and Mapping (PTAM)                                                  &keyframe  &indirect &\cite{klein_2007_ISMAR}\\
				\hline
				2007&Monocular SLAM as a Graph of Coalesced Observations
                &filter      &indirect &\cite{eade_2007_ICCV}\\
				\hline
				2007&Mapping Large Loops with a Single Hand-Held Camera
                &filter      &indirect &\cite{clemente_2007_RSS}\\
				\hline
				2007&Dimensionless Monocular SLAM
                &filter      &indirect &\cite{civera_2007_PRIA}\\
				\hline
				2008&A Square Root UKF for visual monoSLAM&filter&indirect&\cite{holmes_2008_PAMI}\\
				\hline
				\rowcolor{gray}
				2008&An Efficient Direct Approach to Visual SLAM
                &keyframe  &direct   &\cite{silveira_2008_TRO}\\
				\hline
				2008&Efficient View-Based SLAM Using Visual Loop Closures&filter&indirect&\cite{mahon_2008_TRO}\\
				\hline
				2008&Large-Scale SLAM Building Conditionally Independent Local Maps: Application to Monocular Vision&filter&indirect&\cite{pinies_2008_TRO}\\
				\hline
				2009&Towards a robust visual SLAM approach: Addressing the challenge of life-long
                operation &filter      &indirect &\cite{hochdorfer_2009_ICAR}\\
				\hline
				2009&Monocular vision SLAM for indoor aerial
                vehicles&filter&indirect&\cite{celik_2009_IROS}\\
				\hline
				2009&Use a Single Camera for Simultaneous Localization And Mapping with Mobile Object Tracking in dynamic environments&filter&indirect&\cite{migliore_2009_ICRA}\\
				\hline
				\rowcolor{gray}
				2009&Keyframe-based real-time camera tracking&keyframe&indirect&\cite{dong_2009_IJCV}\\
				\hline
				2010&On Combining Visual SLAM and Visual Odometry                                           &filter      &indirect &\cite{williams_2010_ICRA}\\
				\hline
				\rowcolor{gray}
				2010&Scale Drift-Aware Large Scale Monocular SLAM
                &keyframe  &indirect &\cite{strasdat_2010_MIT}\\
				\hline
				\rowcolor{gray}
				2010&Live dense reconstruction with a single moving camera & keyframe &hybrid &\cite{newcombe_2010_CVPR}\\
				\hline
				2010&Monocular SLAM with locally planar landmarks via geometric rao-blackwellized
                particle filtering on Lie groups&filter&indirect&\cite{kwon_2010_CVPR}\\
				\hline
				\rowcolor{gray}
				2011&Dense Tracking and Mapping (DTAM)
                &keyframe  & direct  &\cite{newcombe_2011_ICCV}\\
				\hline
				\rowcolor{gray}
				2011&Omnidirectional dense large-scale mapping and navigation based on meaningful
                triangulation&keyframe&direct  &\cite{pretto_2011_ICRA}\\
				\hline
				\rowcolor{gray}
				2011&Continuous localization and mapping in a dynamic world (CD SLAM)
                &keyframe  &indirect &\cite{pirker_2011_IROS}\\
				\hline
				\rowcolor{gray}
				2011&Online environment mapping&keyframe&indirect&\cite{lim_2011_CVPR}\\
				\hline
				\rowcolor{gray}
				2011&Homography-based planar mapping and tracking for mobile phones&keyframe&indirect&\cite{pirchheim_2011_ISMAR}\\
				\hline
				\rowcolor{gray}
				2013& Robust monocular SLAM in Dynamic environments (RD SLAM)                               &keyframe  &indirect &\cite{tan_2013_ISMAR}\\
				\hline
				\rowcolor{gray}
				2013& Handling pure camera rotation in keyframe-based SLAM (Hybrid SLAM) &keyframe & indirect &\cite{pirchheim_2013_ISMAR}\\
				\hline
				2013&Monocular Vision SLAM for Indoor Aerial
				Vehicles&filter&indirect&\cite{celik_2013_JECE}\\
				\hline
				\rowcolor{gray}
				2013&MonoFusion: Real-time 3D reconstruction of small scenes with a single web camera&keyframe&hybrid&\cite{pradeep_2013_ISMAR}\\
				\hline	
			\end{tabular}
			\end{center}
		\end{table}
	\end{singlespace}
	\restoregeometry
	   \newgeometry{left=1.5cm,bottom=2cm,top=1.5cm}
	   \definecolor{gray}{rgb}{0.75, 0.75, 0.75}
	   \begin{singlespace}
	   	\begin{table*}[!htb]
	   		\centering
	   		\caption{List of different visual SLAM system. Keyframe-based approaches are highlighted in a gray
	   			color continued.}\label{tab:allcontributions2}
	   		\centering
	   		\begin{tabular}{c p{9cm} c c l }
				\hline
				\rowcolor{gray}
				2014&Efficient keyframe-based real-time camera
                tracking&keyframe&indirect&\cite{dong_2014_IJCV}\\
				\hline
				2014&Visual SLAM for Handheld Monocular
                Endoscope&filter&indirect&\cite{grasa_2014_TMI}\\
				\hline
				2014&Real-time camera tracking using a particle filter combined with unscented
                Kalman filters&filter     &indirect &\cite{lee_2014_JEI}\\
				\hline
				\rowcolor{gray}
				2014& Semi-direct Visual Odometry (SVO)
                &keyframe  &hybrid   &\cite{forster_2014_ICRA}\\
				\hline
				\rowcolor{gray}
				2014& Large Scale Direct monocular SLAM (LSD SLAM)
                &keyframe  &direct   &\cite{engel_2014_ECCV}\\
				\hline
				\rowcolor{gray}
				2014& Deferred Triangulation SLAM (DT SLAM)
                &keyframe  &indirect &\cite{herrera_2014_IC3DV}\\
				\hline
				\rowcolor{gray}
				2014&Real-Time 6-DOF Monocular Visual SLAM in a Large Scale
                Environment&keyframe&indirect&\cite{lim_2014_ICRA}\\		   			
	   			\hline
				2015&StructSLAM: Visual SLAM With Building Structure
                Lines&filter&indirect&\cite{zhou_2015_TOVT}\\
				\hline
				\rowcolor{gray}
				2015&Robust large scale monocular Visual SLAM
                &keyframe  &indirect &\cite{bourmaud_2015_CVPR}\\
				\hline
				\rowcolor{gray}
				2015& ORB SLAM &keyframe &indirect &\cite{mur-artal_2015_TRO}\\
				\hline
				\rowcolor{gray}
				2015&Dense Piecewise Parallel Tracking and Mapping (DPPTAM)                                 &keyframe &direct   &\cite{concha_2015_IROS}\\
				\hline
				\rowcolor{gray}
				2016&Multi-level mapping: Real-time dense monocular SLAM&keyframe &hybrid
                &\cite{greene_2016_ICRA}\\
				\hline
				\rowcolor{gray}
				2016&Robust Keyframe-based Monocular SLAM for Augmented Reality&keyframe &indirect
                &\cite{liu_2016_ISMAR}\\
				\hline
				\rowcolor{gray}
				2016&Direct Sparse Odometry&keyframe &direct  &\cite{engel_2016_ARXIV}\\
				\hline
				\end{tabular}
			\end{table*}
		\end{singlespace}
		\restoregeometry
